# Supplementary material for: Hierarchical Functionality Prioritization in Multicast ISAC: Optimal Admission Control and Discrete-Phase Beamforming
Source: arXiv:2501.00201 source file (2024-12-31)
Supplement: Supplementary file 1 [file appendices.tex]

% !TeX root = ../main.tex

\appendix
\section{Appendix} \label{appendix}

This is an appealing appendix.
